# Supplementary material for: Divide and Conquer: Rethinking the Training Paradigm of Neural Radiance Fields
Source: arXiv:2401.16144 source file (2024-01-29)
Supplement: Supplementary file 1 [file X_suppl.tex]

\clearpage
\setcounter{page}{1}
\maketitlesupplementary

\section{Community detection}
In this section, we discuss the community detection algorithms and empirically justify our design choice of Louvain community detection. The following text will introduce the Louvain community detection~\cite{blondel2008fast} and the spectral clustering algorithm~\cite{ng2001spectral}.
\subsection{Louvain community detection}\label{subsec:louvain}
The Louvain community detection algorithm starts by establishing each node as an individual community, denoted as ${\mathcal{P}_1, \ldots, \mathcal{P}_N}$. The algorithm evaluates the modularity gain achievable by relocating a specific node, $I_i$, into various communities, represented as $\mathcal{P}_j$. If the relocation results in an increased modularity gain\footnote{Modularity gain is computed by: 
$\Delta Q=\frac{k_{i,in}}{2m} - \gamma\frac{\sum_{tot}\cdot k_i}{2m^2}$, where $m = \frac{1}{2}\sum_{ij}\mathbf{A}_{ij}$, $k_i=\sum_{j}\mathbf{A}_{ij}$, $k_{i,in}$ is the sum of the weights of the links from node $i$ to nodes in the current community of interest $\mathcal{P}_j$, $\sum_{tot}$ is the sum of the weights of the links incident to nodes in $\mathcal{P}_j$, and $\gamma$ is the community resolution parameter.}, the node $I_i$ is then reassigned to the corresponding community $\mathcal{P}_j$. This iterative process continues until no further improvement in modularity can be attained. Following this phase, the algorithm consolidates the communities formed earlier into distinct super nodes, constituting a higher level of organization within the graph. These super nodes are then treated as new communities, initiating a new cycle of the algorithm by assigning each node to these newly formed super nodes. This cyclic procedure allows for progressive refinement of community structures within the network based on modularity optimization. The number of communities $K$ is empirically chosen by controlling the resolution parameter. 

\subsection{Spectral clustering}\label{subsec:sc}
One of the advantages of employing the spectral clustering algorithm lies in its difference from the assumptions in traditional clustering algorithms, such as K-Means~\cite{ahmed2020k}, which presume data points are spherical around each cluster's centers. In contrast, Spectral clustering treats input data as a graph without making assumptions on the form of the data clusters. It begins by constructing an adjacency matrix $\mathbf{A}$ that represents the similarity between data points. Then, an eigenvalue decomposition is performed on $\mathbf{A}$ to form a matrix $\mathbf{X}$, better capturing the input data's inherent structure. In the transformed space, a normalization is employed to ensure each row of $\mathbf{X}$ have unit length. Finally, the conventional clustering techniques, such as K-Means, can be employed to $\mathbf{X}$ to identify clusters. 

\section{Histogram loss}
In this section, we provide the details of the histogram loss~\cite{barron2022mip} employed in our DaC training paradigm. To ensure $P_{\theta_\star}$ produce valid sampled points for $R_{\theta_\star}$, we follow the practice in our baseline model~\cite{fridovich2023k} and mip-NeRF 360~\cite{barron2022mip} to formulate the problem as aligning two histograms with distinct bins, emitted by $P_{\theta_\star}$ $(\mathbf{t}_\star,\mathbf{\alpha}_\star)$ and $P_{\theta_{\mathds{1}_{\mathcal{P}}}}$ $(\mathbf{t}_{\mathds{1}_{\mathcal{P}}}, \mathbf{\alpha}_{\mathds{1}_{\mathcal{P}}})$, where $\mathbf{t}$ is the vector distance from the ray origin (Note that the histogram is constructed by ($\mathbf{t},\textbf{w}$) in~\cite{barron2022mip}). Such a loss function is built under the assumption that a non-zero loss can only be incurred if it is impossible that both histograms are drawn from the same probability distribution  of mass~\cite{barron2022mip}. To achieve so, we define a function that computes the sum of all $\alpha$ values that overlap with interval $T$:
\begin{equation}\label{eqn:bound}
    \text{bound}(\mathbf{t},\mathbf{\alpha},T) = \sum_{T\cap T_j \neq \emptyset}~\mathbf{\alpha}_j.
\end{equation}
Thereby, it must hold that $\alpha_{\mathds{1}_{\mathcal{P}_i}} \leq \text{bound}(\mathbf{t}_{\star}, \mathbf{\alpha}_{\star}, T_i)$ if two histograms are consistent with each other. Finally, the histogram loss employed in our conquer phase can be defined as:
\begin{equation}\label{eqn:histo}
    \mathcal{L}_{\text{hist}} = 
    \sum_i \frac{1}{\alpha_{\mathds{1}_{\mathcal{P}_i}}} \max(0,\alpha_{\mathds{1}_{\mathcal{P}_i}} - \text{bound}(\mathbf{t}_{\star},\alpha_\star, T_i)).
\end{equation}
Please refer to~\cite{barron2022mip} and~\cite{fridovich2023k} for more comprehensive details regarding the loss functions employed in our DaC framework. 

\section{Additional implementation details}
In this section, we include additional implementation details of our DaC training paradigm. During our conquer phase, we balance multiple losses with coefficients of 0.4 for color $\mathbf{c}$ point-wise loss, 0.3 for $\alpha$ point-wise loss, and 0.3 for histogram loss. Notably, we observe that these coefficients not only stabilize the distillation process but also achieve optimal performance in the context of our experiments. 

In specific scenarios, both the Louvain community and spectral clustering algorithms fail to produce even-sized subgroups. To address this challenge, we opt for a more straightforward approach utilizing percentile division. In the case of 4 subgroups, we partition the input views based on their azimuthal angle into quartiles: 0-25th percentile, 25th-50th percentile, 50th-75th percentile, and 75th-100th percentile. This method guarantees the generation of even-sized subgroups during the dividing phase. We implement this strategy as an initialization of the Louvain community detection for the M60 and Truck of Tanks\&Temples dataset.
